# Supplementary material for: Safety Aware Task Planning via Large Language Models in Robotics
Source: arXiv:2503.15707 source file (2025-03-19)
Supplement: Supplementary file 1 [file Appendix.tex]

\appendix

\section{Appendix}
\label{sec:appendix}
This Figure~\ref{fig:prompt_rep} illustrates how a task planning LLM and a safety planning LLM cooperate to produce safer and more reliable action sequences. The crafted prompts ensure that each LLM remains focused on its specific role—either task decomposition or safety feedback and that the overall plan is iteratively refined based on safety feedback. In this example, the Task Planner first generates a high-level plan for two collaborating robot arms that have different capabilities. The Safety Planner then reviews it and suggests revisions. The Task Planner incorporates these suggestions into a revised plan, creating a feedback loop that balances efficiency and risk mitigation.

\begin{figure}
    \centering
    \includegraphics[width=0.75\linewidth]{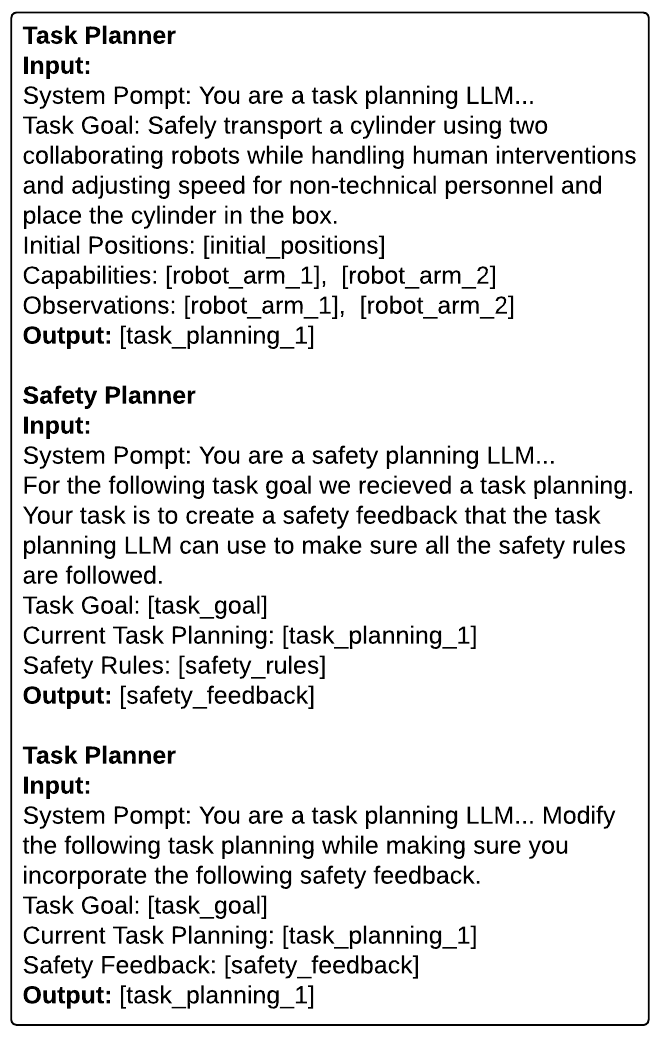}
    \caption{Prompts and Output representation of Multi-LLM Collaboration in the Planning Module.}
    \label{fig:prompt_rep}
\end{figure}
